# Supplementary material for: Full-conformal novelty detection
Source: arXiv:2501.02703 source file (2026-10-29)
Supplement: Supplementary file 1 [file supplement.tex]

\documentclass[12pt]{article}
\input{preamble}

% Import main-text labels; PDF links follow the submission folder layout.
\externaldocument[][nocite]{main}[../kfcnd_main.pdf]
\begin{document}
\spacingset{1}
\appendix

% Distinguish supplemental objects from those in the main text.
\renewcommand{\theequation}{S\arabic{equation}}
\renewcommand{\thefigure}{S\arabic{figure}}
\renewcommand{\thetable}{S\arabic{table}}
\renewcommand{\thealgocf}{S\arabic{algocf}}
\renewcommand{\thedefinition}{S\arabic{definition}}
\renewcommand{\thetheorem}{S\arabic{theorem}}
\renewcommand{\thelemma}{S\arabic{lemma}}
\renewcommand{\thetrick}{S\arabic{trick}}
\renewcommand{\theproperty}{S\arabic{property}}
\renewcommand{\theexample}{S\arabic{example}}
\renewcommand{\thecorollary}{S\arabic{corollary}}
\renewcommand{\theremark}{S\arabic{remark}}
\renewcommand{\theassumption}{S\arabic{assumption}}
\renewcommand{\theproposition}{S\arabic{proposition}}

\begin{center}
{\Large\bfseries Full conformal novelty detection}\\[2ex]
{\large\bfseries SUPPLEMENTARY MATERIAL}
\end{center}
\input{./sections/appendix}
\clearpage
\bibliographystyle{apalike}
\bibliography{ref}
\end{document}
